# Supplementary material for: First electrical White Rabbit absolute calibration inter-comparison
Source: arXiv:2201.08640 source file (2022-01-21)
Supplement: Supplementary file 1 [file Appendix.tex]

\section{Appendix}
\label{App:Appendix}

\subsection{mode abscal losing lock}
It has been observed that command mode abscal should \textbf{always} be executed (i.e. obtain an external 10 MHz phase re-lock) each time the SFP loopback is (re-)inserted.
Failing to do so may lead to invalid and improper measurement results!

Faulty measurements can be recognized by the non-Gaussian shape of the TIC\textsubscript{t1} histogram and a severe increase in the standard deviation.
Figure~\ref{fig:histogram_example} shows an example of a proper- (figure~\ref{fig:app_proper_histogram}, $\sigma$ = 13.69 ps) and a failing-histogram (figure~\ref{fig:app_fail_histogram}, $\sigma$ = 152.93 ps).

A proper measurement (figure~\ref{fig:app_proper_TIC_t1_minus_WR_t1}) shows a \enquote{\textbf{constant}} TIC\textsubscript{t1}. For a failing measurement TIC\textsubscript{t1} is \textbf{not} constant, as can be seen in figure~\ref{fig:app_failing_TIC_t1_minus_WR_t1}.
Moreover, there is a strong correlation with the \enquote{TIC\textsubscript{PPS $\rightarrow$ abscal\_txts} and WR\textsubscript{t1}} (see figure~\ref{fig:app_failing_TIC_t1_WR_t1}) and the TIC\textsubscript{t1} (figure~\ref{fig:app_failing_TIC_t1_minus_WR_t1}) measurement.

A hypothesis for this behavior is that the WR Soft-PLL lost lock and the Soft-PLL is somehow influenced by the pace at which PTP-Sync messages are generated by the software. 

\begin{figure}[htbp]
	\centering
	\begin{subfigure}{.5\textwidth}
		\centering
		\includegraphics[width=1\linewidth]{Appendix/CLBv3_meas_2/Historam_TICt1.png}
		\caption{Proper}
		\label{fig:app_proper_histogram}
	\end{subfigure}%
	\begin{subfigure}{.5\textwidth}
		\centering
		\includegraphics[width=1\linewidth]{Appendix/CLBv3_meas_3/Historam_TICt1.png}
		\caption{Failing}
		\label{fig:app_fail_histogram}
	\end{subfigure}
	\caption{Example of a TIC\textsubscript{t1} histogram for a proper and a failing measurement.}
	\label{fig:histogram_example}
\end{figure}

\begin{figure}[htbp]
	\centering
	\begin{subfigure}{1\textwidth}
		\centering
		\includegraphics[width=1\linewidth]{Appendix/CLBv3_meas_2/Time_Interval_Counter_and_WR_t1,_t4p_versus_measurement_number.png}
		\caption{TIC\textsubscript{PPS $\rightarrow$ abscal\_txts} and WR\textsubscript{t1} measurement.}
		\label{fig:app_proper_TIC_t1_WR_t1}
	\end{subfigure}
	\begin{subfigure}{1\textwidth}
		\centering
		\includegraphics[width=1\linewidth]{Appendix/CLBv3_meas_2/WR_t1_deviation_from_TIC_value.png}
		\caption{TIC\textsubscript{PPS $\rightarrow$ abscal\_txts}$-$WR\textsubscript{t1} = \textbf{\textit{constant}} = TIC\textsubscript{t1}.}
		\label{fig:app_proper_TIC_t1_minus_WR_t1}
	\end{subfigure}
	\caption{Proper \enquote{constant} TIC\textsubscript{t1} measurement.}
	\label{fig:Proper_TIC_t1_measurement}
%\end{figure}

%\begin{figure}[htbp]
%	\centering
	\begin{subfigure}{1\textwidth}
		\centering
		\includegraphics[width=1\linewidth]{Appendix/CLBv3_meas_3/Time_Interval_Counter_and_WR_t1,_t4p_versus_measurement_number.png}
		\caption{TIC\textsubscript{PPS $\rightarrow$ abscal\_txts} and WR\textsubscript{t1} measurement.}
		\label{fig:app_failing_TIC_t1_WR_t1}
	\end{subfigure}
	\begin{subfigure}{1\textwidth}
		\centering
		\includegraphics[width=1\linewidth]{Appendix/CLBv3_meas_3/WR_t1_deviation_from_TIC_value.png}
		\caption{TIC\textsubscript{PPS $\rightarrow$ abscal\_txts}$-$WR\textsubscript{t1} = \textbf{\textit{\textcolor{red}{not} constant}} = TIC\textsubscript{t1}.}
		\label{fig:app_failing_TIC_t1_minus_WR_t1}
	\end{subfigure}
	\caption{Failing TIC\textsubscript{t1} measurement. Note the correlation between the figures where TIC\textsubscript{t1} should have been constant.}
	\label{fig:Failing_TIC_t1_measurement}
\end{figure}

\subsection{Mode abscal PTP\_SYNC message out of synchronisation with PPS signal}
wrpc-sw.git

% October 13, 2020: proposed_master SHA-1: 36c333f
\enquote{* Define NS\_PER\_CLOCK=16 for WR\_NODEs that have CONFIG\_WR\_NODE\_PCS16 set.
Repairs mode abscal that failed to send PTP\_SYNC after each PPS on CLB.}

\subsection{Abscal Tx timestamp signal in wrong clock domain}
A bug was found and fixed in the time-stamping unit\footnote{wr-cores.git ep\_timestamping\_unit.vhd. Bug repair with commit
% October 13, 2020: peter_201007a SHA-1: 0697cbe
\enquote{* Splitted the tx\_timestamp signal in two clock domains; refclk for phys output, sysclk for lm32}.}.
The abscal\_txts signal existed in the system clock domain (clk\_sys, used by the LM32 embedded CPU) while all timing related signals exist in the reference clock (clk\_ref) domain.
This bug has no effect on the SPEC reference design where both clk\_sys and clk\_ref domains are phase locked.

\subsection{SFP EEPROM access}

By accident CLBv3 was fully calibrated with a gateware file that later turned out failing to be able to access the I2C SFP interface needed for storing the $\Delta$\textsubscript{TXcal} and $\Delta$\textsubscript{RXcal} calibration parameters.

\newpage
